# Supplementary material for: Explainable Spatio-Temporal Graph Neural Networks
Source: arXiv:2310.17149 source file (2023-10-26)
Supplement: Supplementary file 1 [file supplementary.tex]

\section{Supplementary Material}
\balance
\label{sec:supplementary}
\subsection{Related Work}
\noindent\textbf{Spatial-Temporal Prediction.}
Spatial-temporal prediction has been widely concerned by the research community and has many significant real-world applications, \eg, traffic forecasting~\cite{DCRNN,DeepST}, crime prediction~\cite{DeepCrime, ST-SHN} and epidemic forecasting~\cite{covid19,CausalGNN}.
Initially, traditional statistical approaches for time series prediction (\eg, HA~\cite{HA}, SVM~\cite{SVM}) are leveraged for spatial-temporal prediction, treating it as an independent multiple time series prediction. 
Considering the correlations among different spatial instances (\eg, urban regions and sensors), approaches simultaneously modeling spatial and temporal dependencies are proposed. 
According to previous literature~\cite{DL-Traff}, spatial-temporal prediction tasks are generally categorized into two classes, \ie, \emph{graph-based} and \emph{grid-based}. 
As to traffic prediction, Convolutional Neural Networks are typically employed to capture complex spatial correlations\cite{DeepST, ST-ResNet, DMVST-Net,ConvLSTM,ST-MetaNet, UrbanFM} for grid-based traffic flow prediction, while Graph Neural networks (GNN) present a  representation ability for spatial dynamics modeling in spatial-temporal graph forecasting~\cite{DCRNN,STGCN, STMGCN, STGODE, DMSTGCN, GraphWaveNet, MTGNN, ST-GDN}.
Concerning temporal dependencies, Recurrent Neural Networks (RNN)~\cite{DCRNN, STMGCN, DMVST-Net, AGCRN, STDN, ST-MetaNet} and Temporal Convolutional Networks (TCN)~\cite{STGCN, GraphWaveNet, DMSTGCN, MTGNN, ASTGCN, STGODE} are utilized in both sorts of methods. 
Recently, attention mechanism is widely used to capture spatial and temporal correlations~\cite{ST-WA, STDN, GMAN, STCGA}. 
Also, \emph{grid-based} crime prediction intrigues this research community by adopting diverse deep learning techniques, \eg, multi-head self-attention~\cite{DeepCrime, STtrans}, hypergraph neural networks~\cite{ST-SHN} and contrastive learning~\cite{ST-HSL}. \\\vspace{-0.1in}

\noindent\textbf{Explainable Machine Learning on Graphs.}
To provide faithful and human-intelligent explanations for "opening" black-box deep learning models, e\textbf{X}plainability \textbf{A}rtificial \textbf{I}ntelligence (XAI) has been increasingly significant especially when applying in real applications. 
Explainable machine learning on graphs aim to obtain important subgraphs (including important nodes, edges and features) that contribute to the prediction of GNN models the most to help human understand and trust GNN models. 
Based on the comprehensive survey~\cite{XAI4GNN_survey}, explainability methods on GNN are divided into two categories, \ie, \post\ and \intr. 
For \post\ approaches, GNNExplainer~\cite{GNNExplainer} firstly proposes a model-agnostic method for explanations of GNN and the objective of explainability on graphs, whereas PGExplainer~\cite{PGExplainer} parameterizes the explainable networks and provides the global explanations of GNN models. 
Generally, we can also categorize \post\ approach into two classes, \ie, instance-level~\cite{GNNExplainer, PGExplainer, SubgraphX, GraphMask} and model-level~\cite{XGNN}. 
As to \intr\ methods, models based on Information Bottleneck (IB)~\cite{IB_BB, VIB} show their superiority in predictive accuracy and explainability~\cite{GIB, ib-subgraph, GSAT}. 
Moreover, approaches~\cite{DIR, CAttn} according to invariant learning (IL) and causal Inference are also proposed to identify invariant structures in different environments for better explainability and generalization.
